# Supplementary material for: The Dark Energy Survey Supernova Program: Cosmological biases from supernova photometric classification
Source: arXiv:2111.10382 source file (2021-11-19)
Supplement: Supplementary file 1 [file Appendix_nuisance.tex]

\begin{table*}
\begin{tabular}{lrrrrrrrrrrrrrrrr}
\hline
{} &  \multicolumn{4}{c}{$\Delta\alpha/\alpha$ \%} &  \multicolumn{4}{c}{$\Delta\beta/\beta$ \%}  &  \multicolumn{4}{c}{$\Delta\sigma_{\mathrm{Ia, int}}/\sigma_{\mathrm{Ia, int}}$ \% } &  \multicolumn{4}{c}{$S_{\mathrm{non-Ia}}-1$} \\
{} &  Baseline & J17 & DES-CC & Data &  Baseline & J17 & DES-CC & Data &  Baseline & J17 & DES-CC & Data &  Baseline & J17 & DES-CC & Data\\
\hline
1 &         -0.49 &      -0.90 &     -0.42 &        0.00 &        -0.64 &     -1.01 &    -1.15 &       0.00 &          -1.51 &       -1.38 &      -1.73 &         0.00 &        0.01 &     0.71 &    1.06 &     -0.76 \\
2 &         -0.49 &      -0.90 &     -0.42 &        0.00 &        -0.64 &     -1.01 &    -1.15 &       0.00 &          -1.51 &       -1.38 &      -1.73 &         0.00 &        0.01 &     0.71 &    1.06 &     -0.76 \\
3 &         -0.88 &      -1.04 &     -0.99 &        0.52 &        -0.97 &     -0.92 &    -1.30 &      -2.58 &          -1.57 &       -2.11 &      -1.99 &        -4.49 &        0.57 &     0.37 &    1.12 &      1.96 \\
4 &         -0.71 &      -0.94 &     -0.84 &        0.22 &        -0.47 &     -0.49 &    -0.75 &      -2.40 &          -0.83 &       -1.43 &      -1.14 &        -5.09 &       -0.01 &     0.32 &   -0.14 &      0.73 \\
5 &         -0.53 &      -1.04 &     -0.41 &       -0.06 &        -0.74 &     -1.38 &    -1.25 &       0.04 &          -1.03 &       -0.46 &      -1.35 &         0.09 &        0.08 &     0.40 &    1.29 &     -0.73 \\
6 &         -0.97 &      -1.24 &     -0.92 &        0.41 &        -1.15 &     -1.24 &    -1.37 &      -2.85 &          -1.34 &       -1.56 &      -1.59 &        -4.31 &        0.84 &     0.23 &    1.19 &      2.71 \\
7 &         -0.73 &      -1.12 &     -0.82 &        0.23 &        -0.57 &     -0.75 &    -0.77 &      -2.52 &          -0.26 &       -0.54 &      -0.45 &        -4.49 &       -0.02 &     0.04 &   -0.20 &      0.72 \\
8 &          0.68 &       2.70 &      0.95 &        3.57 &         2.00 &      6.60 &     1.49 &      -0.50 &           9.45 &       10.69 &       9.86 &         8.02 &        0.00 &     0.00 &    0.00 &      0.54 \\
9 &          0.63 &       1.14 &      1.11 &        5.35 &        -0.01 &      0.98 &     0.29 &      -2.53 &           7.53 &        7.20 &       7.38 &        -0.43 &        0.00 &     0.00 &    0.00 &     -0.19 \\
\hline
\end{tabular}
\end{table*}
